# Supplementary material for: Intrinsic Quasiparticle Lifetime in a Superconducting Aluminum
Source: arXiv:2411.16614 source file (2024-11-25)
Supplement: Supplementary file 1 [file Supplemental_Material_to_Intrinsic_Quasiparticle_Lifetime_in_Superconducting_Aluminum.pdf]

# "Intrinsic Quasiparticle Lifetime in a Superconducting Aluminum" Supplemental Material

K. Norowski,[1,*] M. Foltyn,[1] A.Savin,[2] M. Zgirski,[1,†]

[1]CoolPhon Group, International Research Centre MagTop, Institute of Physics,
Polish Academy of Sciences, Aleja Lotnikow 32/46, PL 02668 Warsaw, Poland
[2]QTF Centre of Excellence, Department of Applied Physics
Aalto University, FI-00076, Aalto, Finland

To whom correspondence should be addressed:
* norowski@ifpan.edu.pl † zgirski@ifpan.edu.pl.

## 1 Switching thermometry

When biased with current pulse of a sufficient amplitude nanobridges transit from superconducting to normal state, which we refer to as switching. The switching process for narrow range of testing currents has a stochastic character and it is characterized by a temperature dependent probability $P$. We test the structure with a train of the same short current pulses (duration of 10 ns) to determine the switching probability $P$ of the bridge (Fig. S1). The typical train consists of N = 1 000 or 10 000 cycles. By repeating the measurement for various amplitudes $I_t$ of the testing pulses we get $P(I_t)$ dependencies, known for their shape as S curves (Fig. S2). The switching probability can be also traced for a fixed amplitude of the testing pulse but for various bath temperatures $T_0$ yielding $P(T_0)$ S curves (Fig. S3). They define the temperature responsivity of the thermometer (Fig. S4). To obtain the temporal resolution of our thermometry we add to the measuring protocol the heating pulse with amplitude $I_H$ in each cycle of the train, which is intended to switch and overheat the structure above $T_c$. By delaying the testing pulse, we can determine the variation of the switching probability in the transient (Fig. S5).

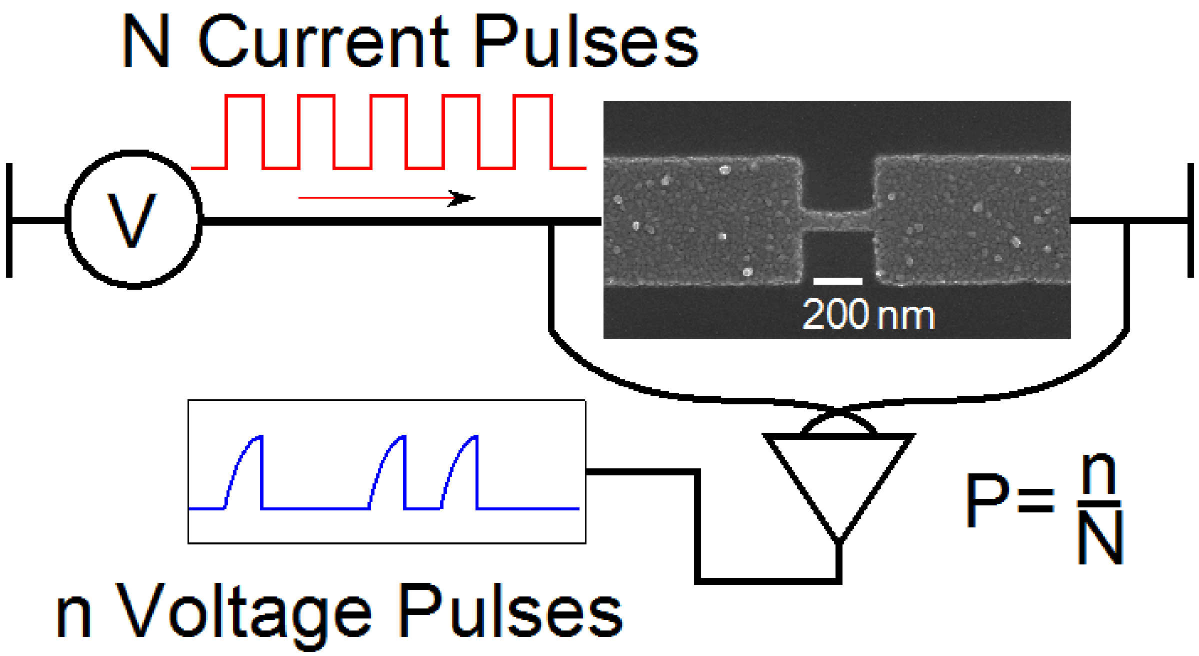


**Figure S1:** Nanobridge probed with $N$ current pulses (each with the same testing amplitude $I_t$) switches $n$ times from a superconducting to normal state yielding switching probability $P = n/N$. The testing current amplitude for which $P = 0.5$ is defined as the switching current $I_{sw}$. The inset is the SEM photo of a representative device studied in this work.

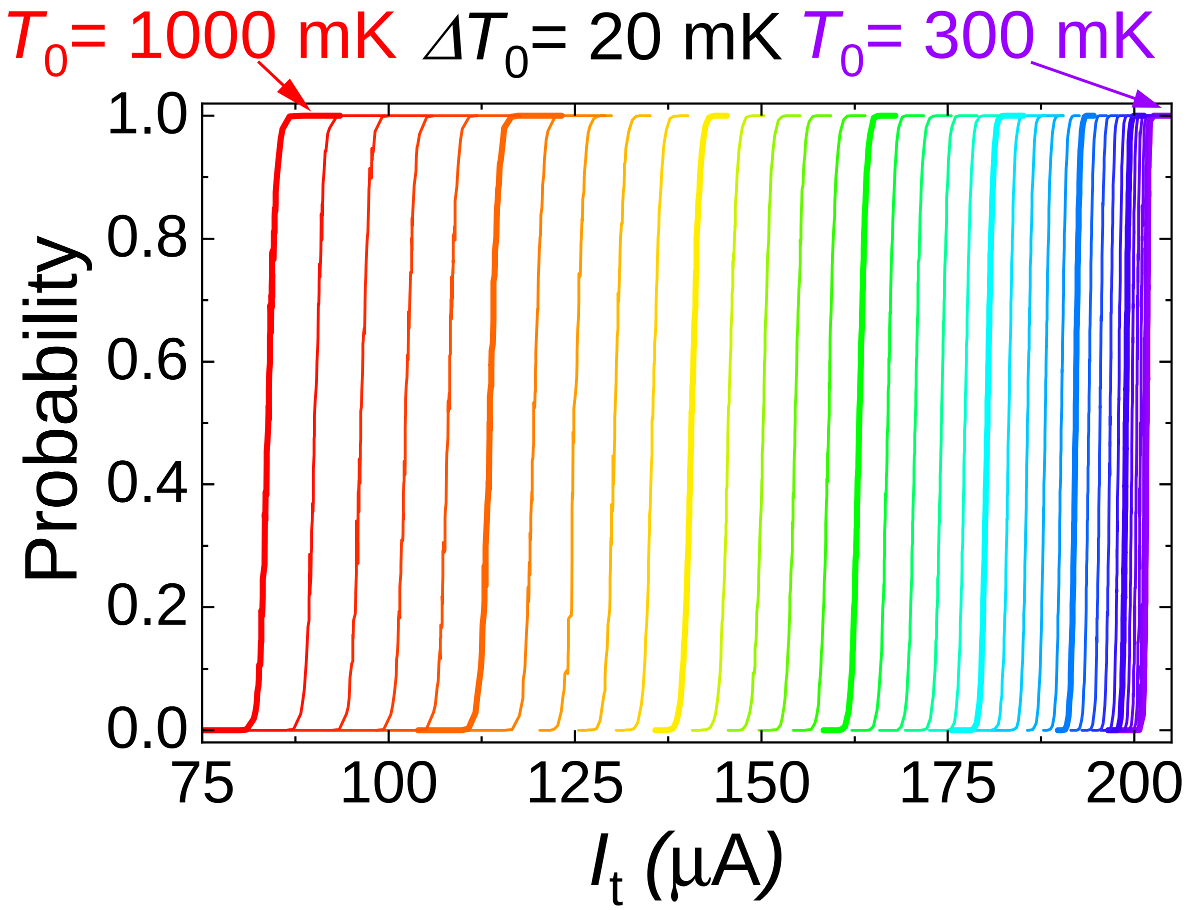


**Figure S2:** The set of S curves recorded at various bath temperatures with step of 20 mK. The value of $I_t$ for which $P = 0.5$ is defined as the switching current $I_{sw}$. The temperature dependence $I_{sw}(T_0)$ calibrates response of the thermometer in dynamic thermal transients in which we monitor temporal variation of $I_{sw}$ [cf. Fig. 2(b)].

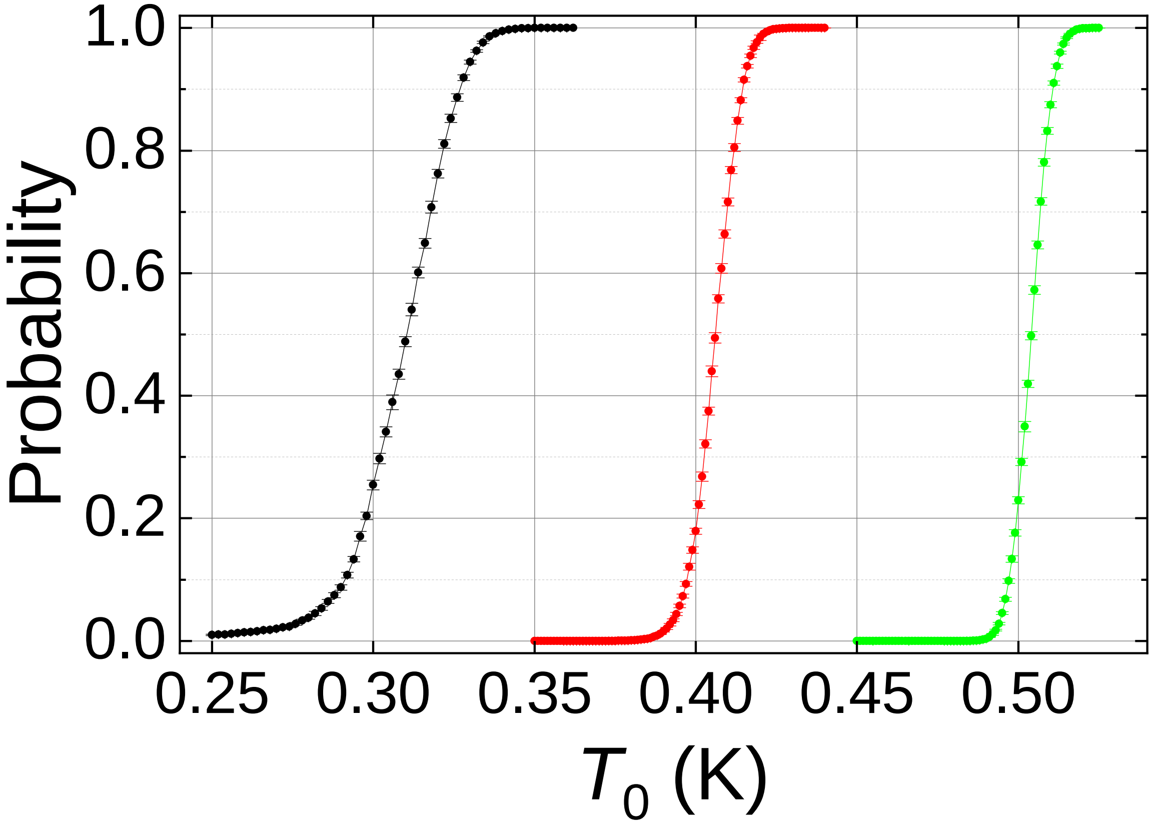


**Figure S3:** The switching probability as a sensitive probe of the local electron temperature. The switching probabilities $P$ vs. the bath temperature $T_0$ for 3 fixed amplitudes of the testing current $I_t$. The slopes of dependencies define the temperature responsivity $dP/dT$ of the thermometer (Fig. S4). At each setpoint $T_0$ probability is measured many times to establish a standard deviation of the measurement, which is presented with the error bars.

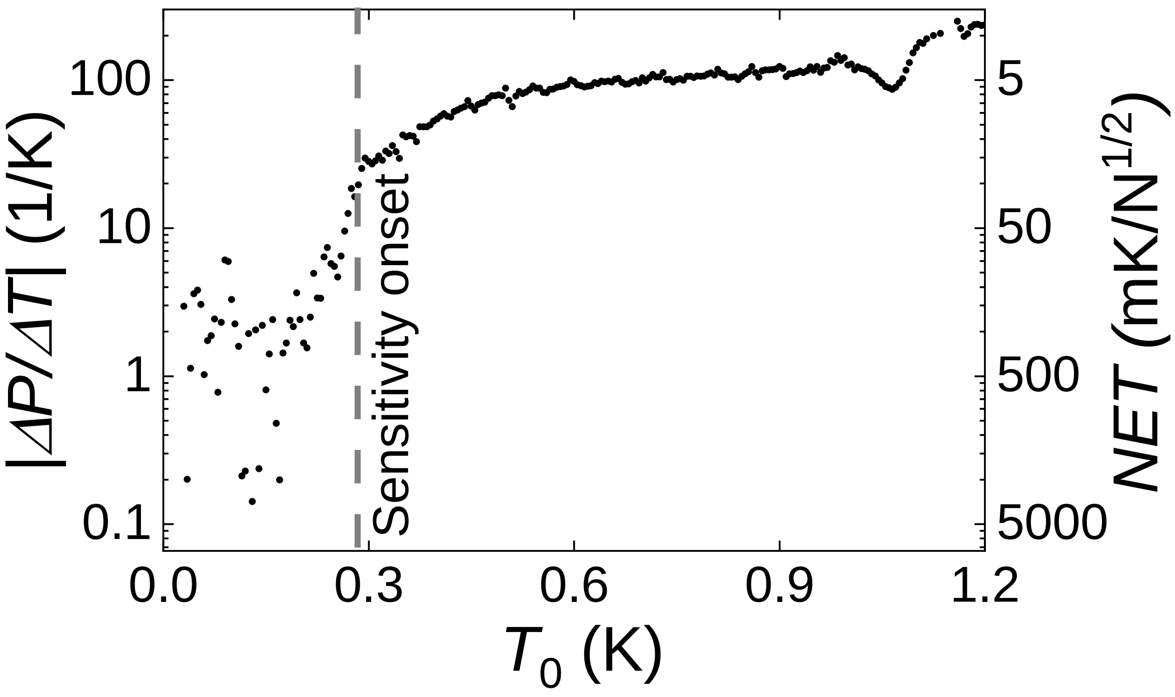


**Figure S4:** The temperature responsivity and the noise-equivalent temperature ($NET$) of the nanobridge. They show flat behavior corresponding to the $NET = 50\,\mu$K for $N = 10\,000$ testing pulses down to $500\,$mK. The scattered characteristics below $280\,$mK marks the operational limit of the thermometer.

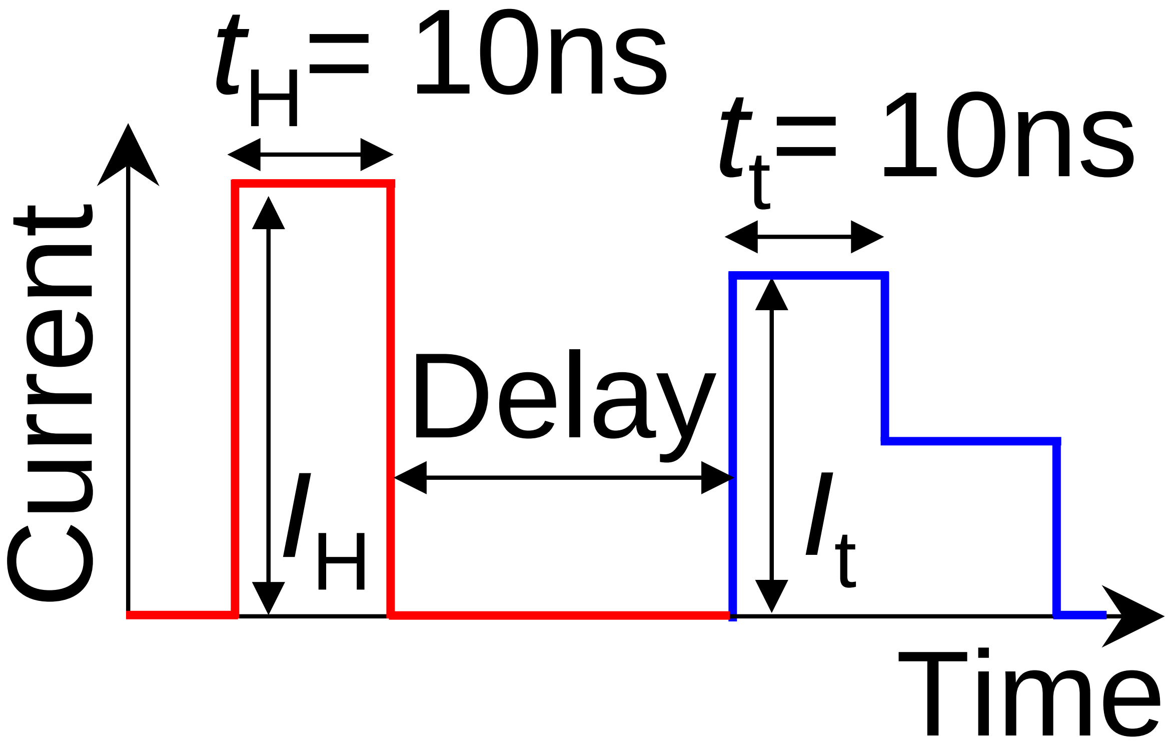


**Figure S5:** The pulse sequence used in the experiment - only one cycle of the train is shown. The first pulse overheats the nanowire above $T_c$, the second pulse is intended to probe the switching probability. The current train consists of $N = 1\,000$ or $10\,000$ such sequences to determine the switching probability for a single delay. In our experiments we use Arbitrary Waveform Generator with bandwidth of 120 MHz, which can deliver 2-3 ns-long rising and trailing edges of the pulses.

## 2 Requirements for a fast and sensitive thermometer

Generally, if we define $P$ as a temperature-sensitive parameter measured in the experiment, the variation of the temperature in the range $(T_0, T_0 + \Delta T)$ places $P$ in the interval $(P_0, P_0 + \Delta P)$. To properly measure QPs relaxation time $\tau_{qp}$ in the linear regime defined as a time after which the $\Delta T = T - T_0$ drops by factor of $e$, the experimental method should feature the following properties (the list is not exhaustive):

1. The temperature responsivity of the thermometer $dP/dT$ should remain significant in the studied thermal transient covering the interval $(T_0, T_0 + \Delta T)$. It means that $\Delta T$ should be much larger than the Noise-Equivalent Temperature ($NET$). This condition may also be written as $\Delta P \gg (dP/dT) \cdot NET$.

2. The thermometer should provide temporal resolution $\Delta t$ much better than the dynamics of the thermal transient under study.

3. The relaxation time should not suffer from overheating, i.e. not show a power dependence.

All required features are provided in our experiment down to 280 mK.

Ad.1. The aluminum superconducting nanobridge provides the cut-off temperature $T_{cut-off}$ of $250 - 270$ mK (Fig. S6). The ability to measure QP lifetime at the lowest temperatures is limited by the temperature responsivity $dP/dT$ of the detector (Fig. S4). The trial to measure the relaxation at $T_{ph} = T_0 < T_{cut-off}$ would lead to observation of the artifact, underestimating the value of the relaxation time (Fig. S7). In simple words, the sensor saturates at the value corresponding to the cut-off temperature $T_{cut-off}$. For $T_{ph} = T_0 < T_{cut-off}$ the quasiparticle population may still go down, but the saturated sensor is not able to follow the temperature change any more. We note that detectors based on the kinetic inductance [1–3] also show similar low temperature cutoff.

Ad.2. The temporal resolution of our thermometry is defined by the duration of the testing pulse, i.e. 5 ns in our case. It is the time in which the bridge has a chance to switch from superconducting to normal state. For a detailed account of the switching thermometry see [4, 5].

Ad.3. We show in Fig. 1(c) that this condition is also satisfied. It is why we call the measured lifetimes the intrinsic ones.

We can modify our nanothermometer by covering the nanobridge with copper or replacing the material of the bridge with titanium but leaving the leads aluminum. In both cases the critical current of the bridge should be lowered and the bridge is expected to show the temperature responsivity at temperatures lower than 280 mK. Such arrangement would allow to study QP population at the lowest temperatures, which may possibly exceed the value expected in equilibrium by many orders of magnitude [6].

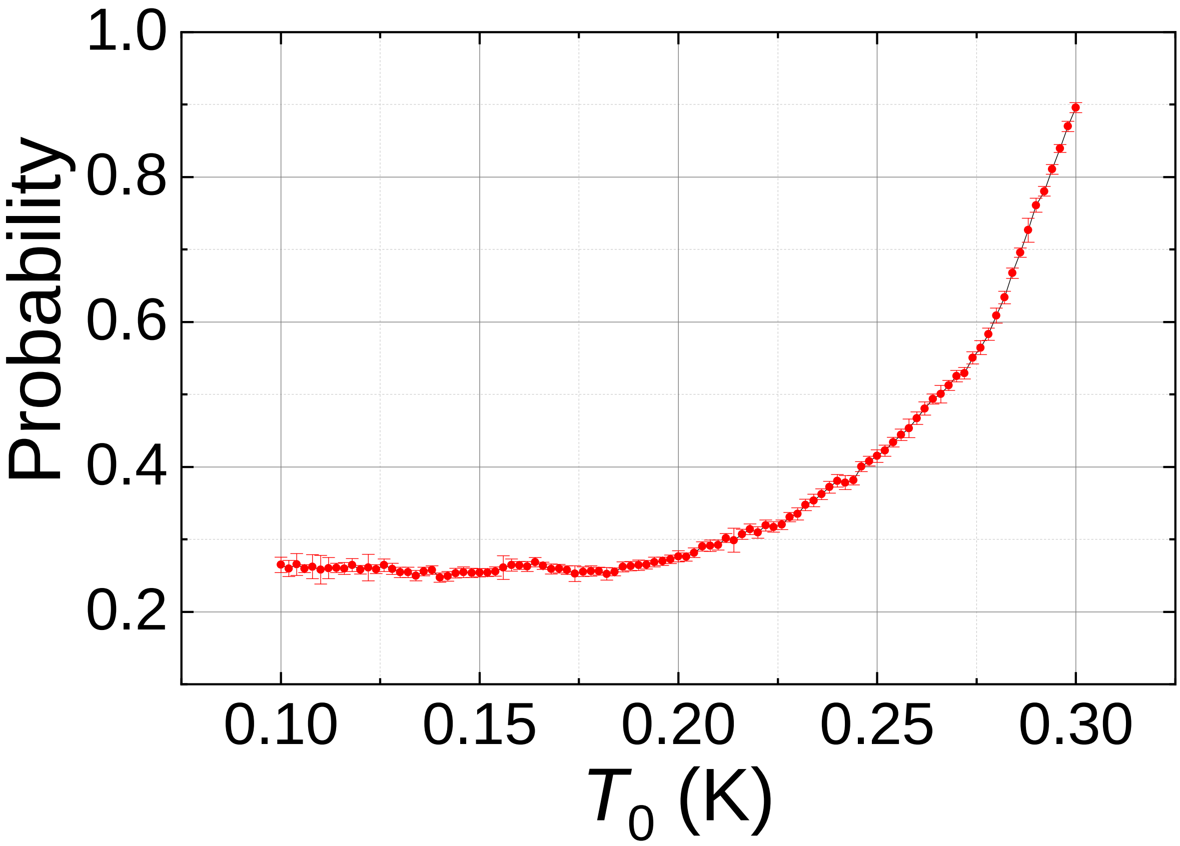


**Figure S6:** The saturation of the switching probability at low temperatures. To see a change in the probability at low temperatures, we choose the testing current yielding $P$= 0.9 at 300 mK. Then the bath temperature is stabilized at fixed setpoints defined with the step of 2 mK. The switching probability is measured many times at each setpoint to establish a standard deviation of the measurement presented here with the error bars.

# 3 The saturation of the relaxation time due to low sensitivity of the thermometer

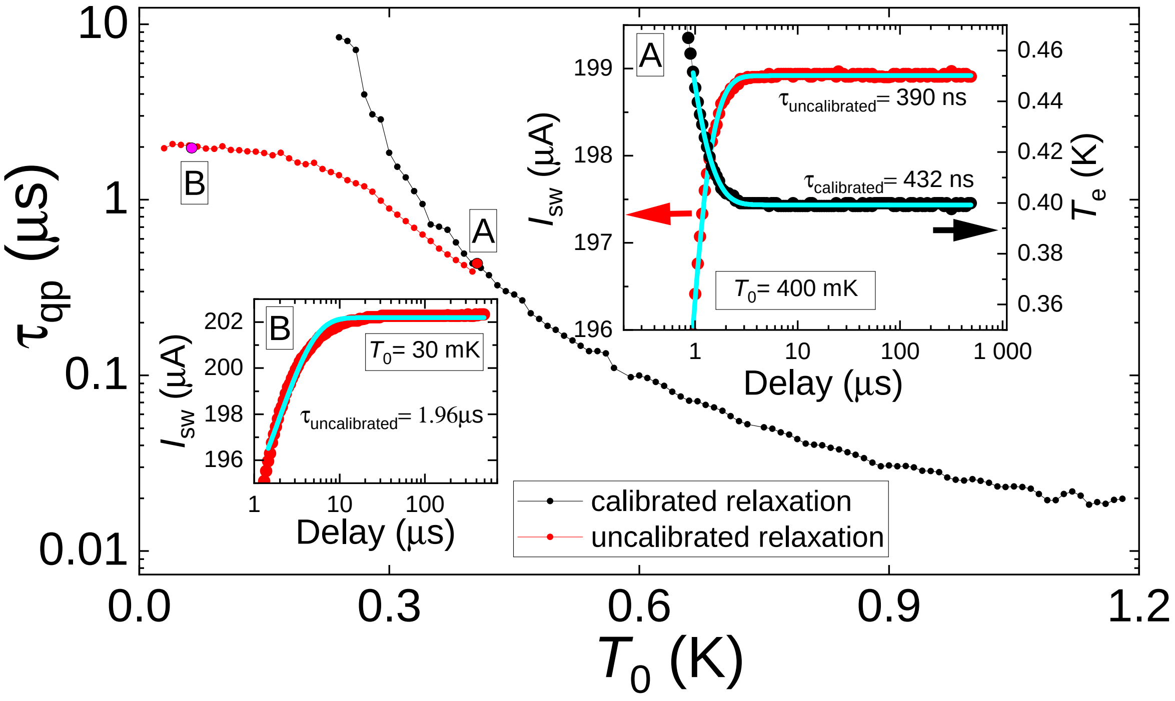


**Figure S7:** The studies of the relaxation time determined using uncalibrated (the relaxation of the switching current) and calibrated (the relaxation of temperature) measurements. Since at low temperatures the switching current $I_{sw}$ hardly changes (cf. Fig. S6), one cannot convert it into temperature. Technically it is still possible to fit the uncalibrated data (inset B shows the relaxation profile collected at $T_0 = 30\,\mathrm{mK}$), but the result vastly underestimates the relaxation time, as linear regime of temperature evolution is not accessible experimentally below $T_{cut-off}$. Such fitting can not give a properly defined relaxation time at $T_0$: $I_{sw}$ saturates when temperature start approaching $T_{cut-off}$ and further cool-down can not be traced experimentally. In contrast, at higher temperatures thermometer remains sensitive, and there is no difference between uncalibrated and calibrated measurement of $\tau_{qp}$ (inset A shows the uncalibrated (left axis) and calibrated (right axis) relaxation profiles collected at $T_0 = 400\,\mathrm{mK}$.

# 4 The thermal properties of a superconducting aluminum - numerical calculations and material parameters

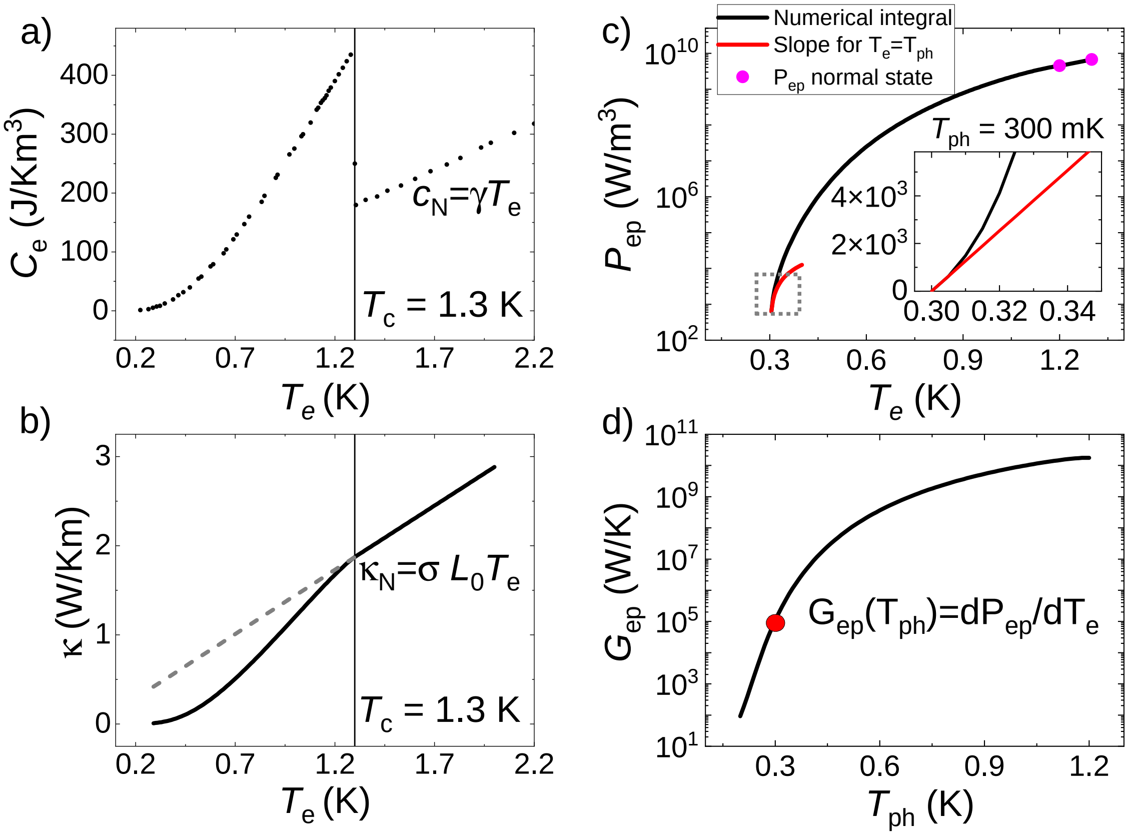


**Figure S8:** Temperature dependencies of the thermal parameters used in modeling. (a) The heat capacity of the aluminum – experimental data extracted from the literature [7]. (b) The electron thermal conductivity – calculated using Eq. S2. Above $T_c$ the dependence is given by the familiar Wiedemann-Franz (WF) law. The gray dashed line is the extension of WF law below $T_c$. (c) Power $P_{ep}$ transmitted to phonons from QPs relaxing to Cooper pairs for phonons kept at $T_{ph} = 300\,\text{mK}$ - result of calculation based on Eq. S1. The calculation at high temperatures merges with values predicted by the power law describing electron-phonon coupling in a normal state i.e $P_{ep} = \Sigma(T_e^5 - T_{ph}^5)$, where $\Sigma = 1.8 \cdot\ 10^9\,\text{Wm}^{-3}\text{K}^{-5}$ (pink points). The red line is the slope $dP_{ep}/dT_e$ at $T_e = T_{ph}$. The inset shows magnified region of the main panel (gray dotted box) in the linear scale. (d) Thermal conductance between electrons and phonons calculated in the linear regime as a derivative $dP_{ep}/dT_e$ at $T_e = T_{ph}$. Here, unlike in panels a, b and c, the horizontal axis refers not to the electron temperature $T_e$ but to the phonon temperature $T_{ph}$. The red point is the slope value extracted for $T_{ph} =\ 300\,\text{mK}$, the case of (c) graph.

Numerical calculation of the heat flow equation (Eq. 1, main text) is executed in the MATLAB PDE toolbox with the superconducting electron-phonon coupling and the superconducting electron thermal conductivity calculated numerically, and by taking heat capacity temperature dependence $C_e(T)$ from literature.

The heat flow from electrons to phonons in the superconducting aluminum was calculated numerically by solving integral[8] [see Fig. S8 (c)]:

$$\begin{aligned} P_{ep} =& \frac{\Sigma_{Al}}{24\xi(5)k_B^5} \int_0^\infty d\epsilon \epsilon^3 \left[n\left(\epsilon, T_S\right) - n\left(\epsilon, T_P\right)\right] \\ &\times \int_{-\infty}^{\infty} dE n_S\left(E\right) n_S\left(E+\epsilon\right) \left(1 - \frac{\Delta^2}{E\left(E+\epsilon\right)}\right) \\ &\times \left[f_S\left(E\right) - f_S\left(E+\epsilon\right)\right] \end{aligned} \qquad \text{(Eq. S1)}$$

where $\Delta$ is the BCS temperature dependent superconducting gap, $\Sigma_{Al} = 1.8{\cdot}10^9\,\mathrm{Wm^{-3}K^{-5}}$ is the material constant for electron-phonon coupling in aluminum, $\xi(z)$-the Riemann zeta function, $n_S(E)$-the BCS density of states, $n(\epsilon, T_P) = \{exp[\epsilon/(k_B T_P)] - 1\}^{-1}$ is the Bose-Einstein distribution of the phonons at temperature $T_P$ and $f_S(E)$ is the Fermi Dirac distribution of quasiparticles.

The electron thermal conductivity in the superconducting state was obtained as a solution of the integral[9] [see Fig. S8 (b)]:

$$\frac{\kappa_S(T)}{\kappa_N(T)} = \frac{3}{2\pi^2} \int_{\Delta/k_B T}^{\infty} \left(\frac{x}{cosh(x/2)}\right)^2 dx \qquad \text{(Eq. S2)}$$

where $\kappa_S(T)$ and $\kappa_N(T)$ are the electron thermal conductivities in the superconducting state and in the normal state respectively. $\kappa_N$ is assumed to follow linear temperature dependence defined by the Wiedemann-Franz law, i.e. $\kappa_N(T) = \sigma T L_0$, where $L_0 = 2.44 \cdot 10^{-8}\,\mathrm{W\Omega K^{-2}}$ is the Lorentz number and $\sigma$ is electrical conductivity ($\sigma_{Al} = 0.5 \cdot 10^8\,\mathrm{S/m}$).

The aluminum heat capacity is determined experimentally in [7] - Fig. S8 (a). Note: $C_P(T_e > T_c) = \gamma T_e$, $\gamma = 135\,\mathrm{JK^{-2}m^{-3}}$ (instead of $91.2\,\mathrm{JK^{-2}m^{-3}}$ expected for the free electron model[10]).

The general expression for resistance of the 1D nanostructure with the nanobridge placed at $x = 0$ is $r(x, T_e) = \frac{\rho(x)}{S}$, where:

$$\rho = \begin{cases} \rho_{Al} & \text{for } T > T_C \\ 0 & \text{for } T < T_C \end{cases}$$

with $\rho_{Al} = 2 \cdot 10^{-8}\,\Omega m$.

# 5 Numerical studies of the interplay of electron-phonon coupling $P_{ep}$ and electron thermal conductivity $\kappa$ in short and long wires

In this section we present some numerical studies of the QP lifetimes $\tau_{qp}$ based on Eq.(1) of the main text. Typical calculated relaxation profiles obtained with the nominal values of the thermal parameters are presented in Fig. S9. Fig. S10 shows the QPs lifetimes in the nanobridge for nominal and rescaled values of the electron-phonon interaction $P_{ep}$ and electron thermal conductivity $\kappa$. Particularly, Fig. S11 demonstrates that by increasing 8 times the strength of the electron-phonon coupling and reducing electron thermal conductivity $\kappa$ by a factor of 4, one can obtain a quantitative agreement between the calculated and measured QP lifetimes both for short and long wires at $T_0 = 300\,\text{mK}$. At higher temperatures ($T_0 > 0.7$ K) nominal values of $P_{ep}$ and $\kappa$ well correspond to the experimentally determined $\tau_{qp}$ (cf. Fig.3).

Fig. S12 shows the comparison of the $\tau_{qp}$ predicted by the Einstein-Smoluchowski law and that obtained by solving the heat flow equation [Eq.(1)] with the only relaxation channel being the electron thermal conductivity.

Fig. S13 presents the nominal calculated timescales of the two energy relaxation channels for QPs: electron-phonon coupling and hot electron diffusion (electron thermal conductance) at different temperatures.

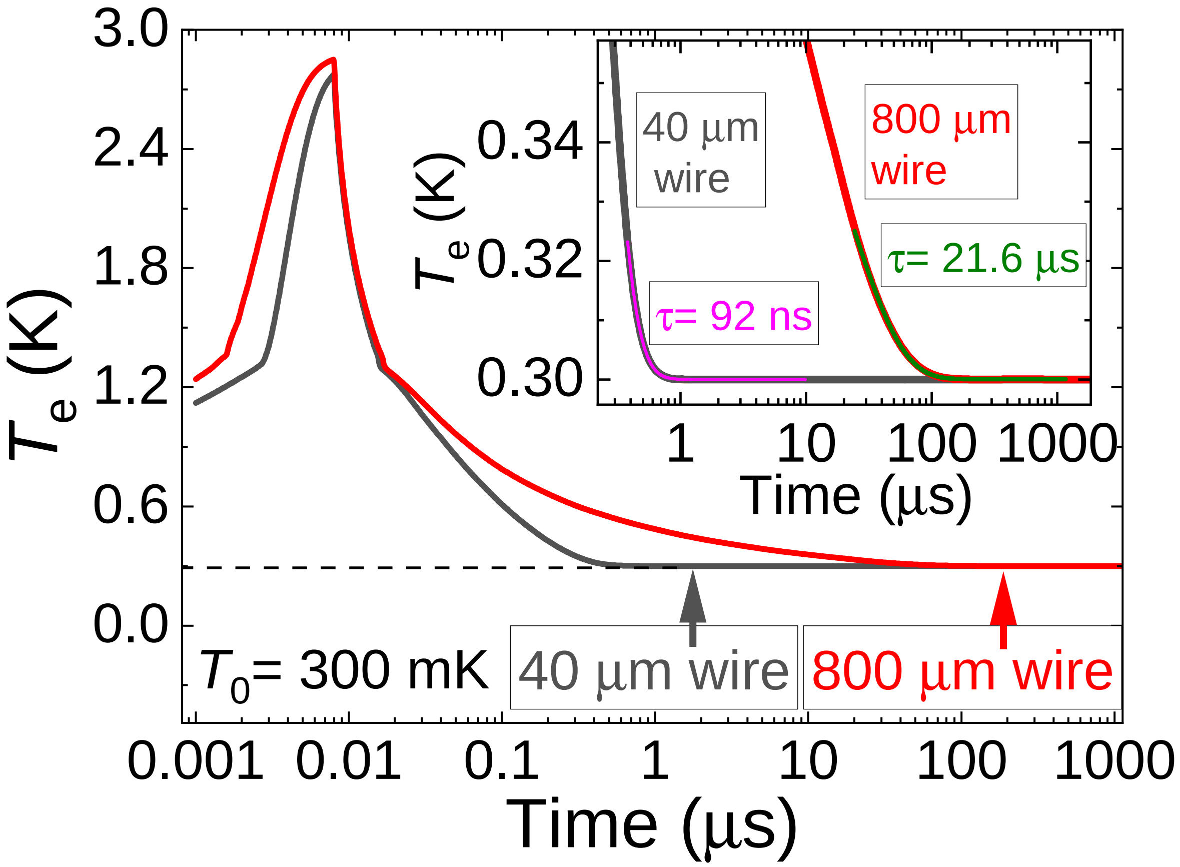


**Figure S9:** The calculated temporal traces of the electron temperature in the nanobridge for long and short wires. The first 10 ns corresponds to duration of the heating pulse which is used to initialize the thermal transient. The inset shows zoomed parts of the curves close to $T_0$ and exponential fits yielding the QP lifetimes.

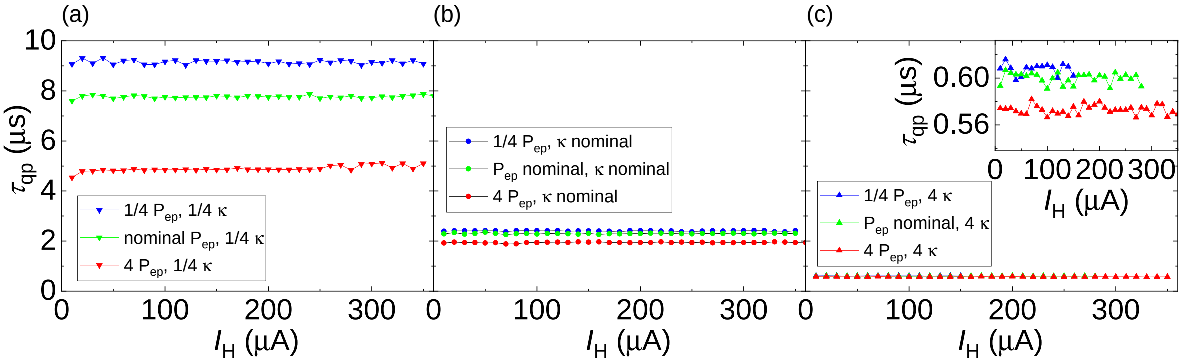


**Figure S10:** QP lifetimes obtained using numerical solution of the 1D heat flow equation [cf. Eq. (1)] for heating pulses of various amplitudes and rescaled values of $P_{ep}$ and $\kappa$. The phonon temperature is assumed to be constant $T_{ph} = T_0 = 300\,\mathrm{mK}$ and the wire length is $200\,\mu\mathrm{m}$. (b,c) In the case of nominal and enhanced $\kappa$ value, the changes in $P_{ep}$ strength hardly modify the $\tau_{qp}$. (a) Conversely, if we suppress $\kappa$, rescaling of $P_{ep}$ starts to be visible. The modeling is insensitive to the heating power i.e. change in the heating current by more than one order of magnitude does not change the lifetime. In general, in experiments a heating of the sample can overheat local sample phonons with respect to the substrate phonons. This effect is not taken into account in our calculation, but Fig.1(c) shows that overheating is not an essential problem in our experiment.

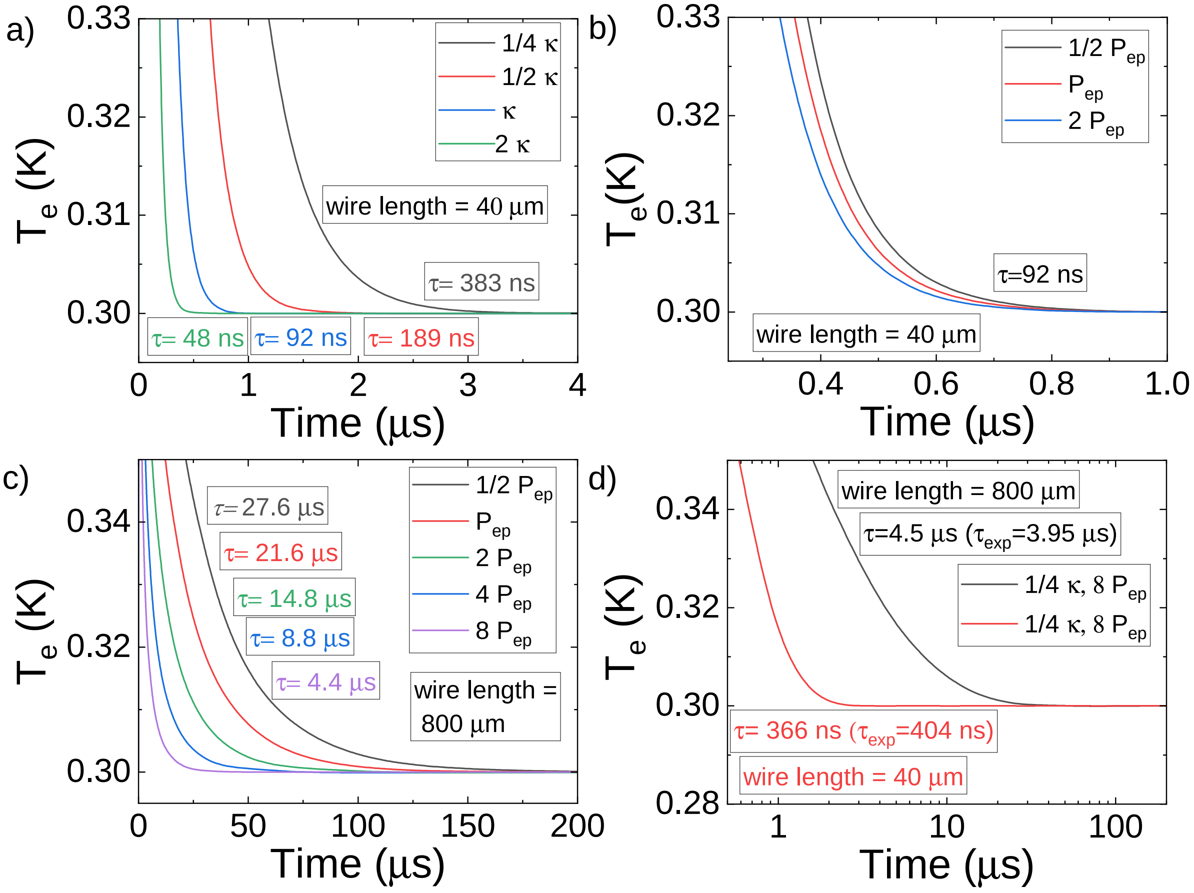


**Figure S11:** The numerical studies of the interplay of electron-phonon coupling $P_{ep}$ and electron thermal conductivity $\kappa$ in short and long wires at $T_0 = 300\,\text{mK}$. (a,b) The relaxation tails for a short wire ($L = 40\,\mu\text{m}$) show sensitivity on the rescaled value of the electron thermal conductivity, but are weakly affected by changes introduced in $P_{ep}$. (c) The relaxations tails of a long wire ($L = 800\,\mu\text{m}$) show sensitivity on the rescaled value of the electron phonon interaction $P_{ep}$. (d) Two relaxation tails, one for short ($L = 40\,\mu\text{m}$) and one for long ($L = 800\,\mu\text{m}$) wire, demonstrate the possibility to adjust the thermal parameters to calculate relaxation times $\tau_{qp}$ which match the experimental lifetimes $\tau_{exp}$ simultaneously for both wires.

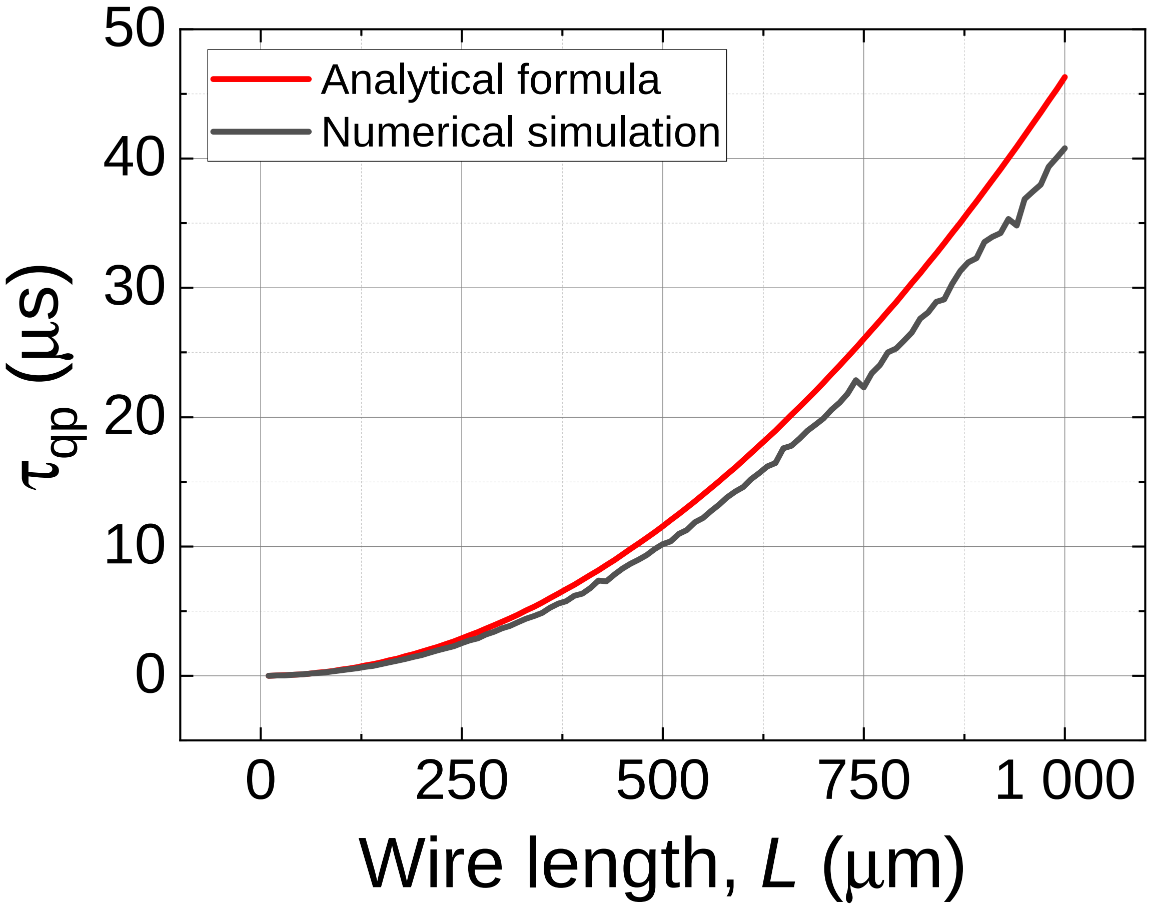


**Figure S12:** The analytical formula for length dependent $\tau_{qp} = \tau_{diff} = \frac{\mathcal{L}^2}{D(T)}$ (where $\mathcal{L} = L/2$), compared to the value obtained from the numerical calculation of the 1D diffusion equation (i.e. Eq. (1). with $P_{ep} = 0$), by fitting the exponential decays to the tails of the temperature relaxations. $T_0 =$ 400 mK. The temperature dependent diffusion coefficient is defined as $D(T) = 2\frac{\kappa(T)}{C(T)}$ [11, 12].

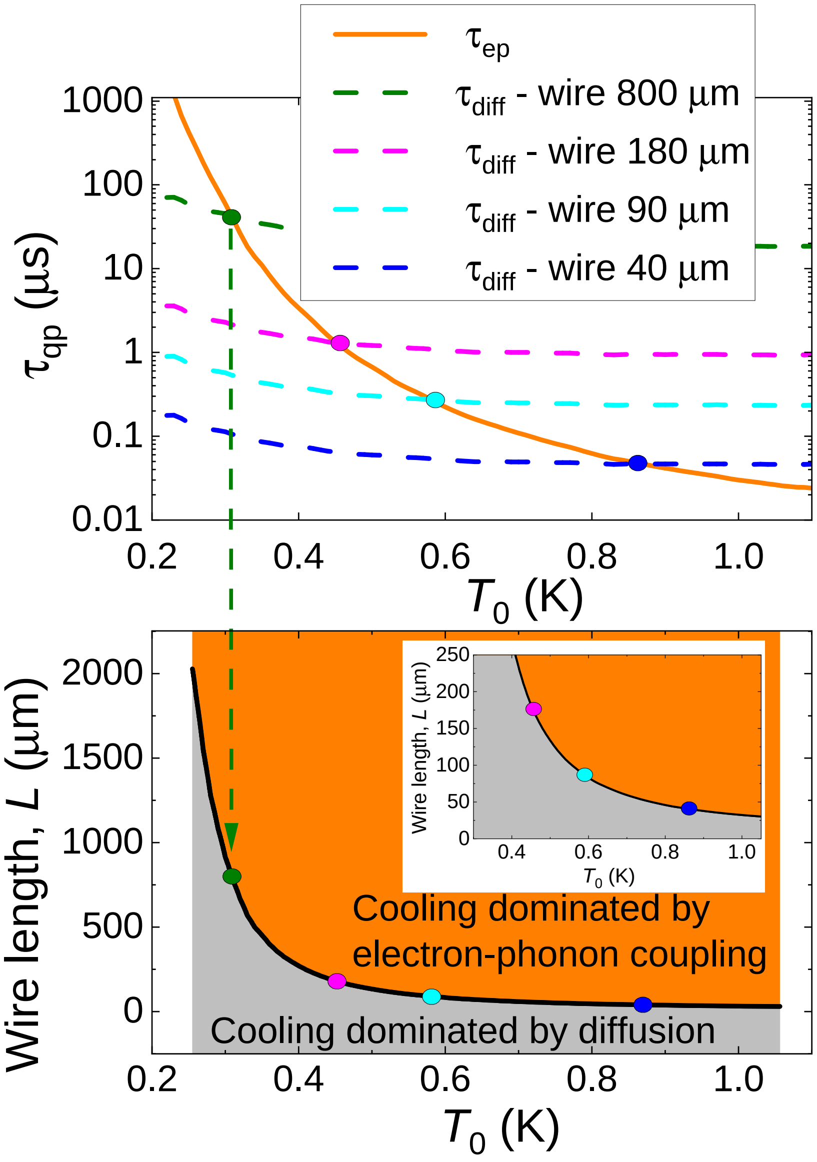


**Figure S13:** The comparison of the temperature dependent timescales of two thermalization mechanisms. The upper graph shows numerically calculated relaxation times due to the electron phonon coupling only (orange line, the same as in Fig.2), and relaxation times resulting exclusively from the diffusion process (dashed lines), calculated using $\tau_{diff} = \frac{\mathcal{L}^2}{D(T)}$ (where $\mathcal{L} = L/2$), with the assumed definition of the temperature dependent diffusion coefficient $D(T) = 2\frac{\kappa(T)}{C(T)}$ [11, 12]. The highlighted points mark length dependent crossover temperature, for which two processes have the same rate. The lower graph shows the diagram of the dominating cooling mechanisms for QPs. The boundary between two regions (black line) was obtained from the requirement $\tau_{ep} = \tau_{diff}$ applied to the different lengths of the wires (green arrow). Above this line, electron phonon coupling dominates ($\tau_{ep} < \tau_{diff}$, orange area) as faster cooling process, and below it the diffusion is more important ($\tau_{ep} > \tau_{diff}$, gray area). This approach is valid assuming that electron phonon coupling and electron diffusion work independently in parallel, i.e. $\frac{1}{\tau_{qp}} = \frac{1}{\tau_{ep}} + \frac{1}{\tau_{diff}}$. Inset of lower graph shows zoom for boundary area at lower wire lengths.

# 6 Experimental QP lifetime for different wire lengths

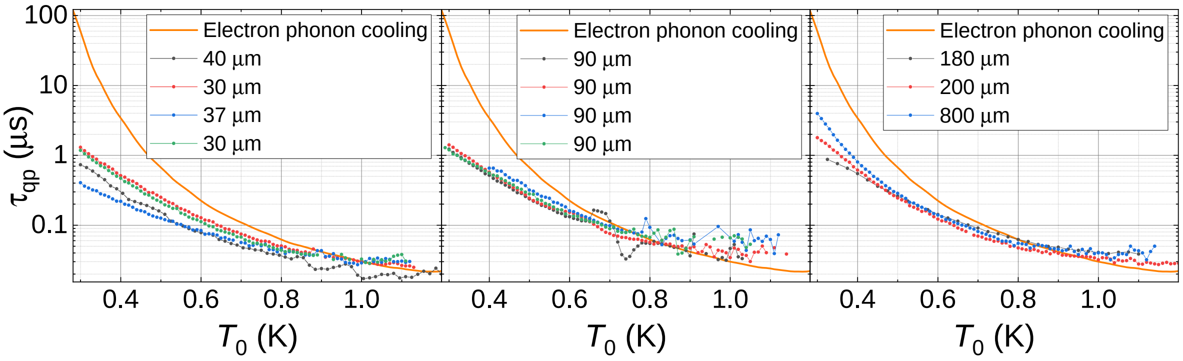


**Figure S14:** QP lifetime vs. bath temperature $T_0$ - sets of experimental data varying by the wire lengths. The orange curve is the reference electron-phonon theory [cf. Eq. (2)]. The longer the wire, the weaker the diffusion contribution to the thermalization process. In consequence, increasing the wire length brings $\tau_{qp}(T)$ closer to the pure electron phonon cooling regime. Regardless of the wire length considered, at high temperatures electron-phonon interaction dominates and the relaxation matches the theory of electron-phonon coupling.

# References and Notes


[1] R. Barends, J. J. A. Baselmans, S. J. C. Yates, J. R. Gao, J. N. Hovenier, and T. M. Klapwijk. Quasiparticle relaxation in optically excited high-$q$ superconducting resonators. *Phys. Rev. Lett.*, 100:257002, Jun 2008. doi: 10.1103/PhysRevLett.100.257002. URL `https://link.aps.org/doi/10.1103/PhysRevLett.100.257002`.

[2] Lukas Grünhaupt, Nataliya Maleeva, Sebastian T. Skacel, Martino Calvo, Florence Levy-Bertrand, Alexey V. Ustinov, Hannes Rotzinger, Alessandro Monfardini, Gianluigi Catelani, and Ioan M. Pop. Loss mechanisms and quasiparticle dynamics in superconducting microwave resonators made of thin-film granular aluminum. *Phys. Rev. Lett.*, 121:117001, Sep 2018. doi: 10.1103/PhysRevLett.121.117001. URL `https://link.aps.org/doi/10.1103/PhysRevLett.121.117001`.

[3] Anthony J Annunziata, Daniel F Santavicca, Luigi Frunzio, Gianluigi Catelani, Michael J Rooks, Aviad Frydman, and Daniel E Prober. Tunable superconducting nanoinductors. *Nanotechnology*, 21(44):445202, oct 2010. doi: 10.1088/0957-4484/21/44/445202. URL `https://dx.doi.org/10.1088/0957-4484/21/44/445202`.

[4] M. Zgirski, M. Foltyn, A. Savin, A. Naumov, and K. Norowski. Heat hunting in a freezer: Direct measurement of quasiparticle diffusion in superconducting nanowire. *Phys. Rev. Appl.*, 14:044024, Oct 2020. doi: 10.1103/PhysRevApplied.14.044024. URL `https://link.aps.org/doi/10.1103/PhysRevApplied.14.044024`.

[5] Marek Foltyn, Konrad Norowski, Alexander Savin, and Maciej Zgirski. Quantum thermodynamics with a single superconducting vortex. *Science Advances*, 10(31): eado4032, 2024. doi: 10.1126/sciadv.ado4032. URL `https://www.science.org/doi/abs/10.1126/sciadv.ado4032`.

[6] Thomas Connolly, Pavel D. Kurilovich, Spencer Diamond, Heekun Nho, Charlotte G. L. Bøttcher, Leonid I. Glazman, Valla Fatemi, and Michel H. Devoret. Coexistence of nonequilibrium density and equilibrium energy distribution of quasiparticles in a superconducting qubit. *Phys. Rev. Lett.*, 132:217001, May 2024. doi: 10.1103/PhysRevLett.132.217001. URL `https://link.aps.org/doi/10.1103/PhysRevLett.132.217001`.

[7] Norman E. Phillips. Heat capacity of aluminum between 0.1°k and 4.0°k. *Phys. Rev.*, 114:676–685, May 1959. doi: 10.1103/PhysRev.114.676. URL `https://link.aps.org/doi/10.1103/PhysRev.114.676`.

[8] V. F. Maisi, S. V. Lotkhov, A. Kemppinen, A. Heimes, J. T. Muhonen, and J. P. Pekola. Excitation of single quasiparticles in a small superconducting al island connected to normal-metal leads by tunnel junctions. *Phys. Rev. Lett.*, 111:147001, Oct 2013. doi: 10.1103/PhysRevLett.111.147001. URL `https://link.aps.org/doi/10.1103/PhysRevLett.111.147001`.

[9] H. Courtois, M. Meschke, J. T. Peltonen, and J. P. Pekola. Origin of hysteresis in a proximity josephson junction. *Phys. Rev. Lett.*, 101:067002, Aug 2008. doi: 10.1103/PhysRevLett.101.067002. URL `https://link.aps.org/doi/10.1103/PhysRevLett.101.067002`.

[10] C. Kittel. *Introduction to Solid State Physics*. Oxford University Press, November 2004. ISBN 978-0-471-41526-8. URL https://www.wiley.com/en-us/Introduction+to+Solid+State+Physics%2C+8th+Edition-p-9780471415268.

[11] Stephen Blundell and Katherine Blundell. *Concepts in Thermal Physics*. Oxford University Press, 10 2009. ISBN 9780199562091. doi: https://doi.org/10.1093/acprof:oso/9780199562091.001.0001. URL https://doi.org/10.1093/acprof:oso/9780199562091.001.0001.

[12] Jack Ekin. *Experimental Techniques for Low-Temperature Measurements: Cryostat Design, Material Properties and Superconductor Critical-Current Testing*. Oxford University Press, 10 2006. ISBN 9780198570547. doi: 10.1093/acprof:oso/9780198570547.001.0001. URL https://doi.org/10.1093/acprof:oso/9780198570547.001.0001.
